# Supplementary material for: Quadratic Zeeman Spectral Diffusion of Thulium Ion Population in a Yttrium Gallium Garnet Crystal
Source: arXiv:2210.05005 source file (2022-10-10)

a.

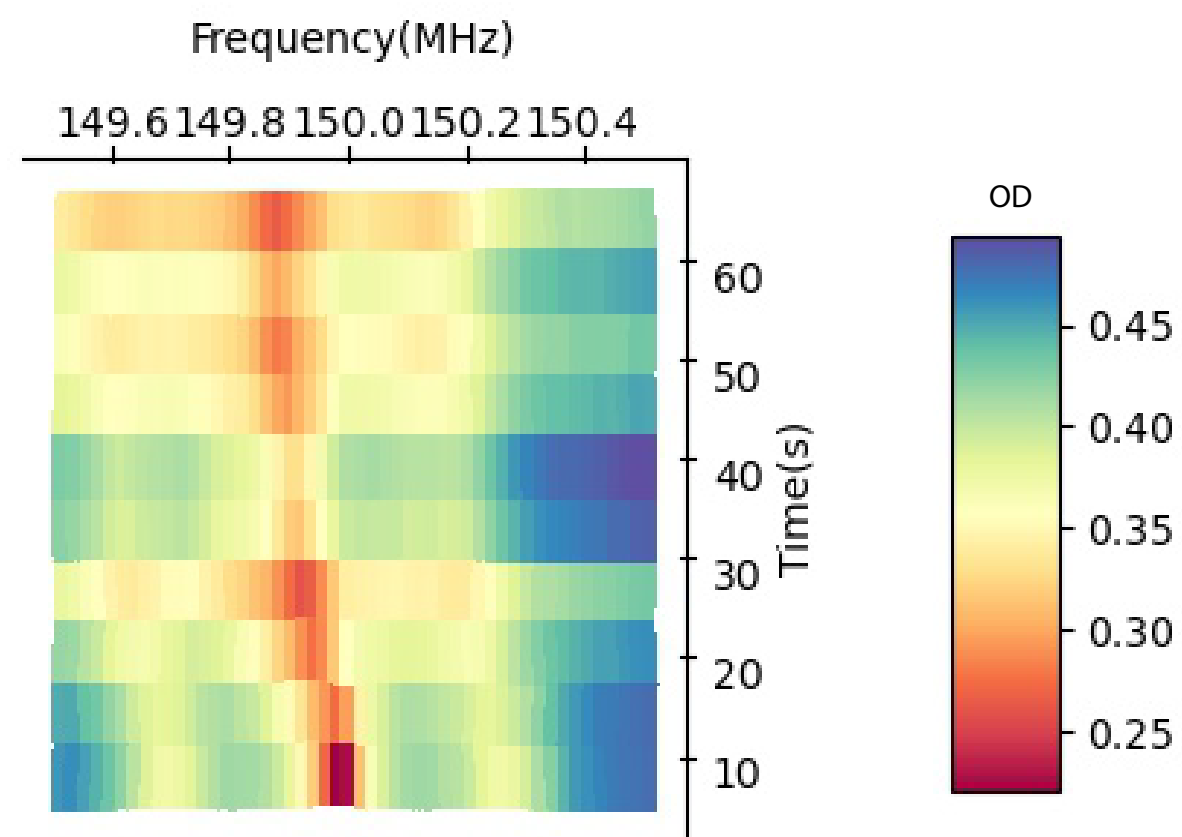

b.

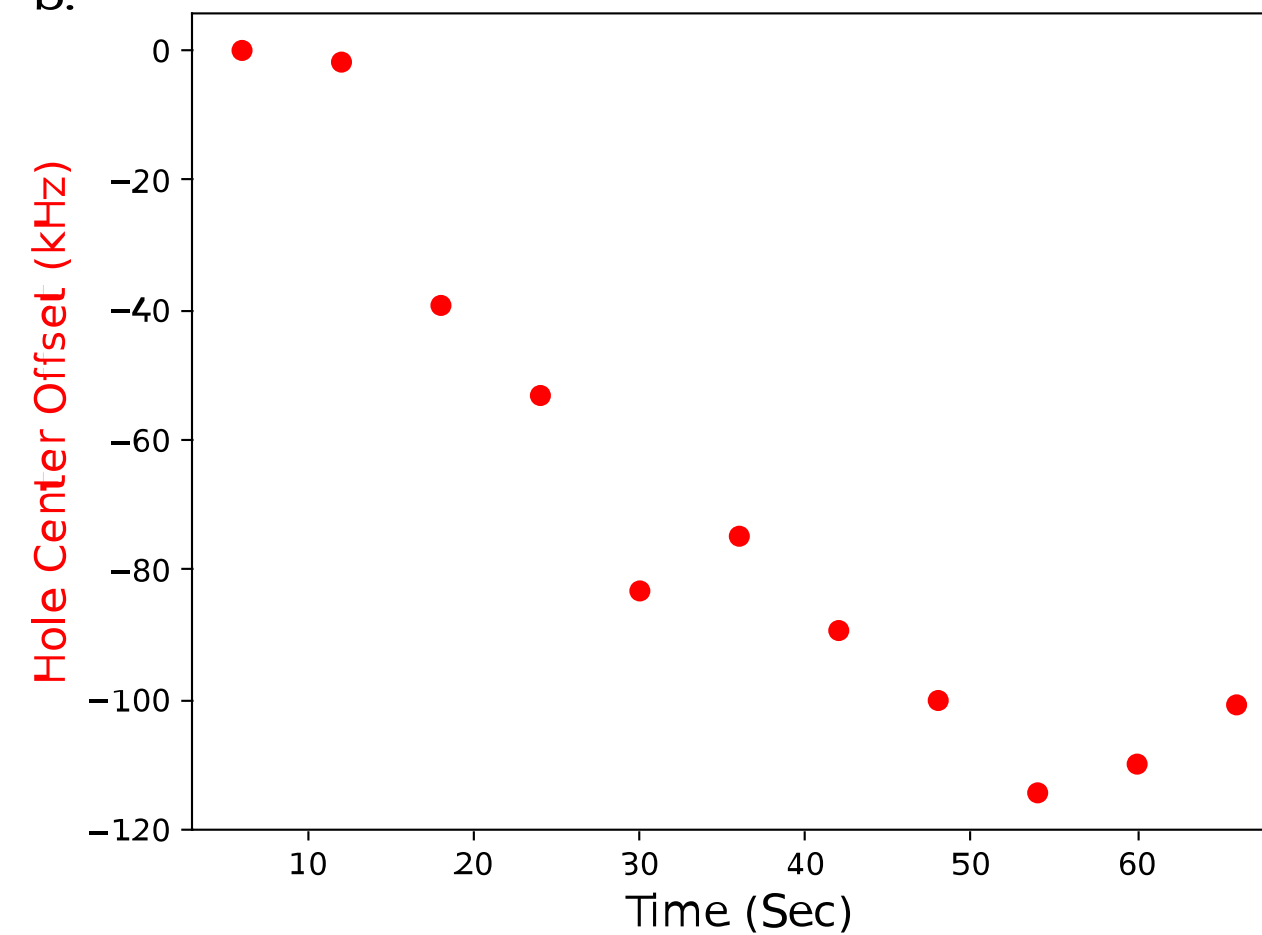

c.

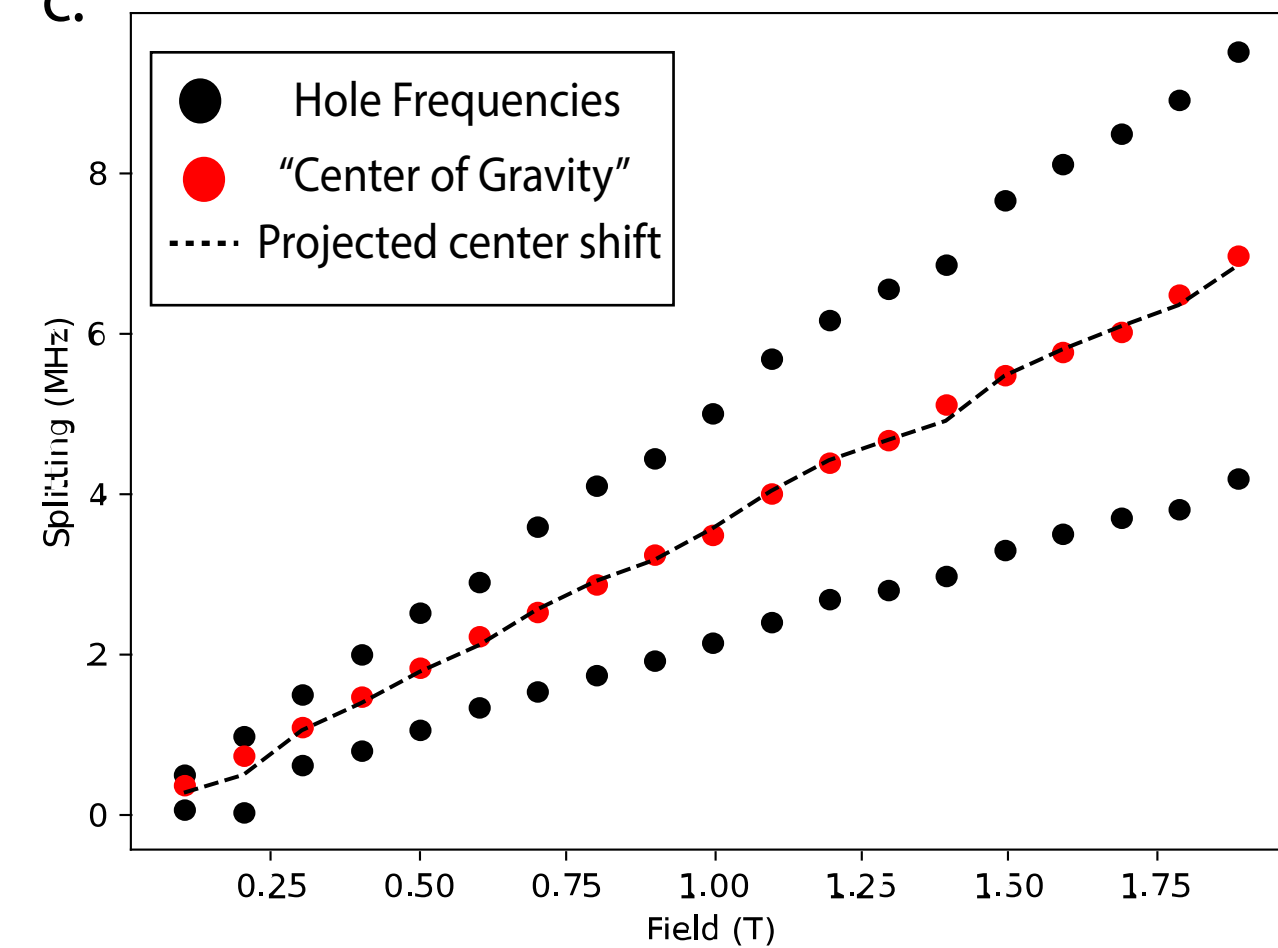

d.

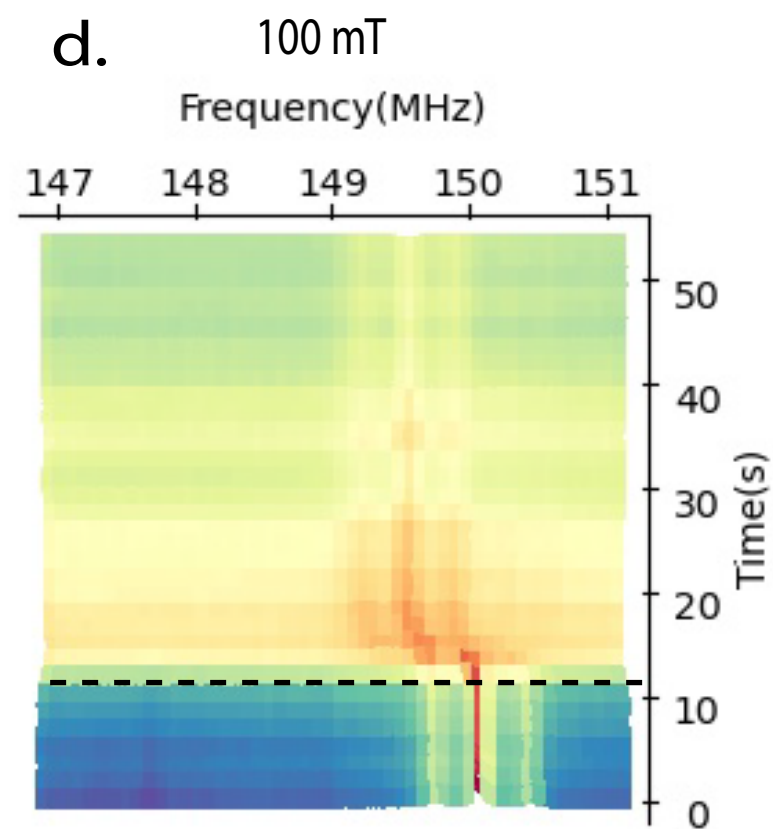

e.

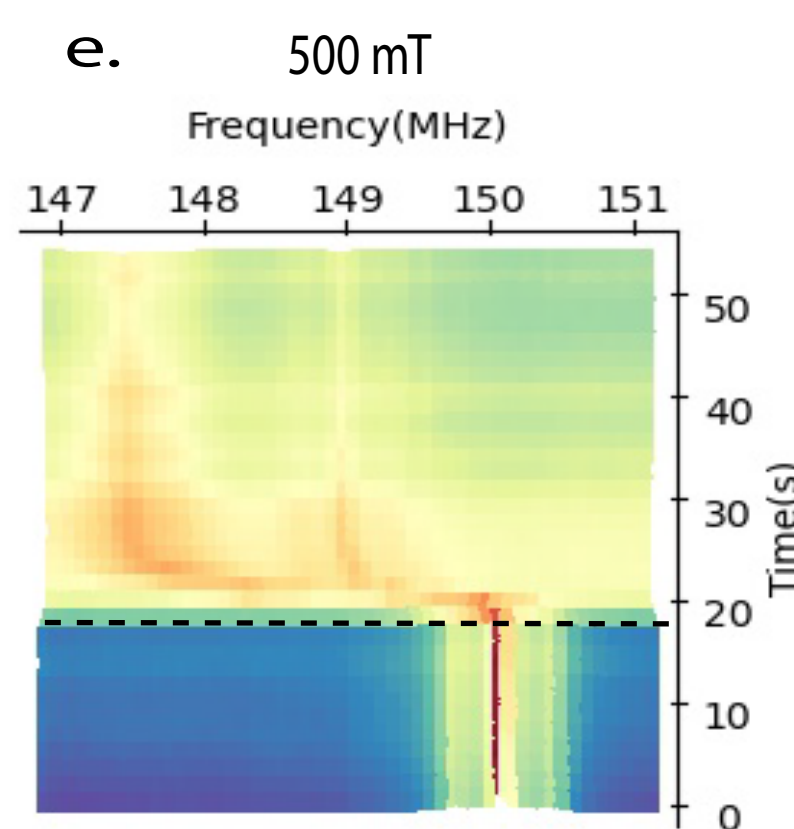

f.

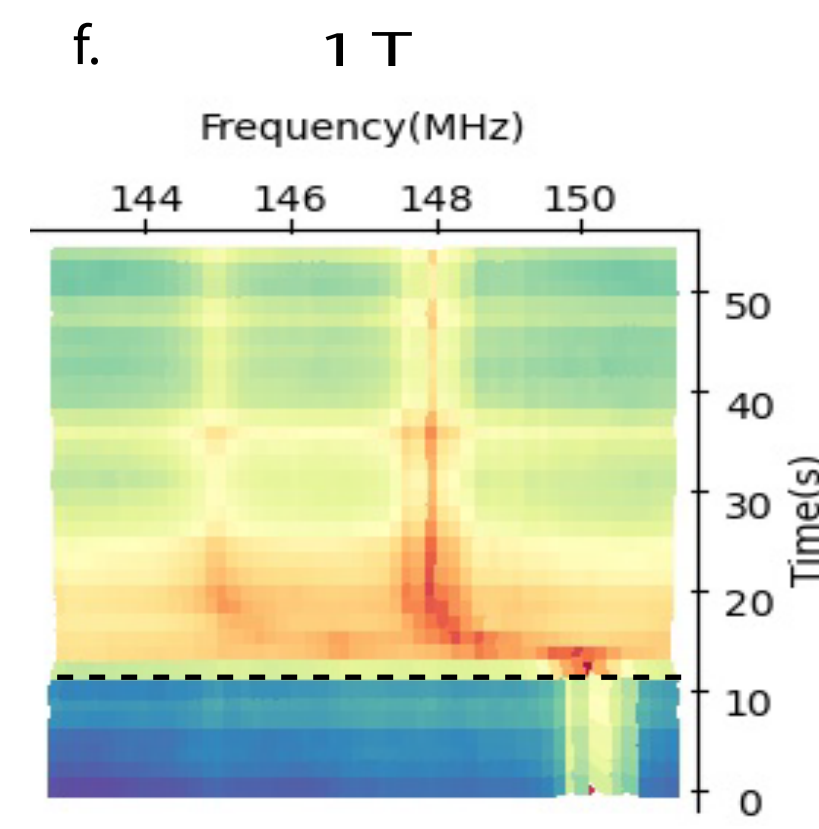

g.

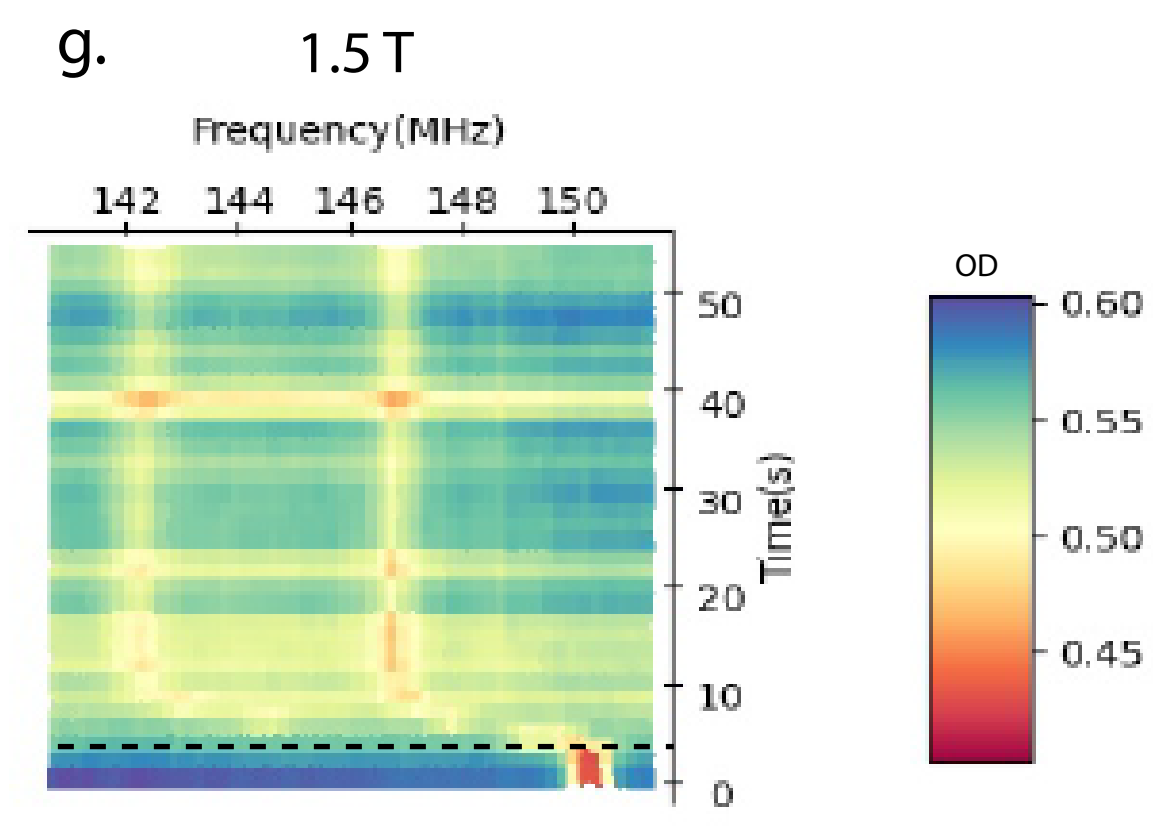

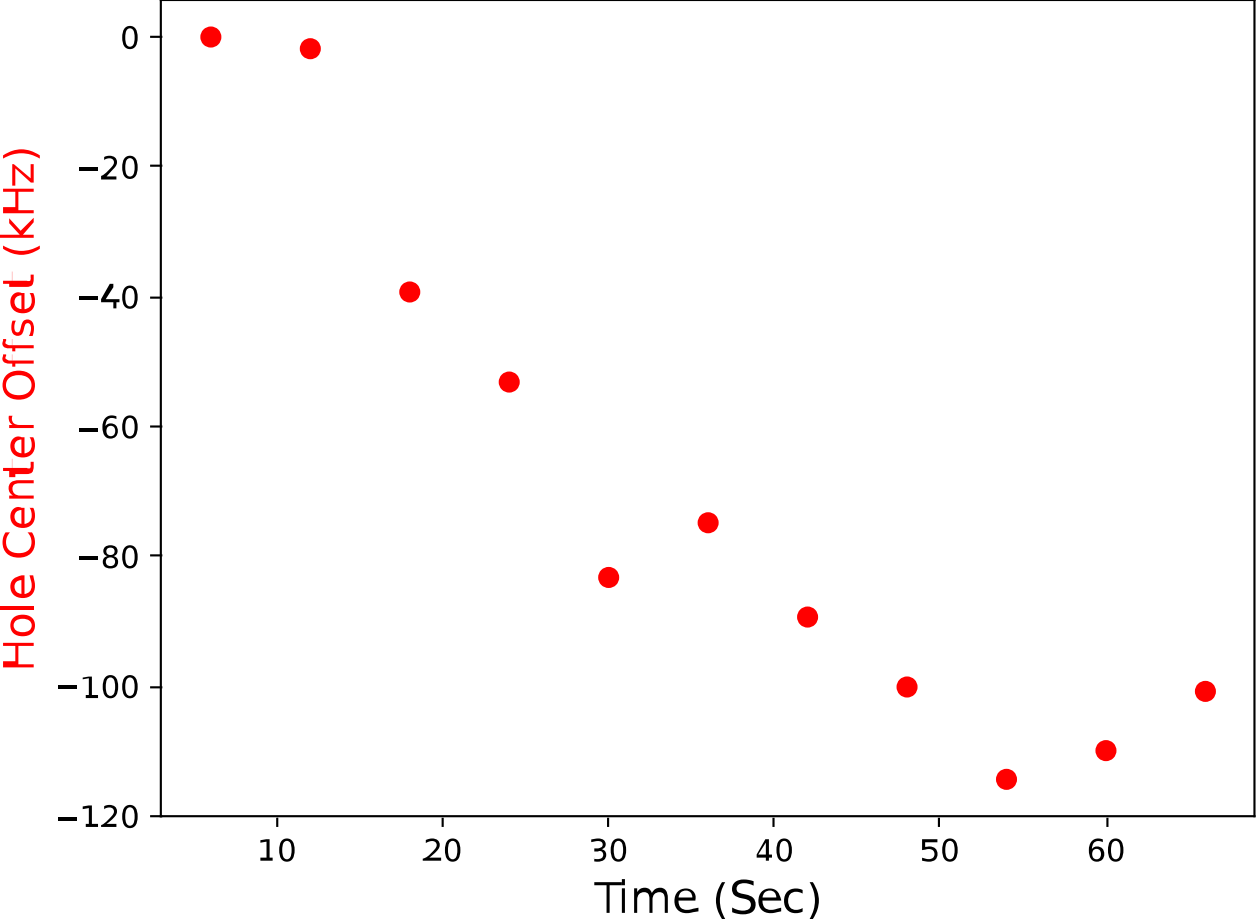

Supplement: Supplementary file 1 [file SI_Magnetic_Noise.pdf]
